# Supplementary material for: Band gaps of hybrid metal halide perovskites: efficient estimation
Source: arXiv:2402.08419 source file (2024-02-13)
Supplement: Supplementary file 1 [file AK13_SI.pdf]

**Band gaps of hybrid metal halide perovskites: efficient estimation**

Sergei M. Butorin

Condensed Matter Physics of Energy Materials, X-ray Photon Science, Department of Physics and Astronomy, Uppsala University, P.O. Box 516, SE-751 20 Uppsala, Sweden

Input files to generate the full relativistic norm-conserving pseudopotentials using ONCVPSP v.4.0.1.

```
# ATOM AND REFERENCE CONFIGURATION
# atsym  z   nc   nv    iexc    psfile
  Pb 82.00  12   3      4      upf
#
#   n   l   f       energy (Ha)
    1   0   2.00
    2   0   2.00
    2   1   6.00
    3   0   2.00
    3   1   6.00
    3   2  10.00
    4   0   2.00
    4   1   6.00
    4   2  10.00
    4   3  14.00
    5   0   2.00
    5   1   6.00
    5   2  10.00
    6   0   2.00
    6   1   2.00
#
# PSEUDOPOTENTIAL AND OPTIMIZATION
# lmax
    3
#
#   l,   rc,     ep,   ncon, nbas, qcut
    0   3.53404   0.00000   5   8   3.96156
    1   3.59528   0.00000   5   8   3.58114
    2   3.28108   0.00000   5   8   6.04705
    3   3.57558   0.26797   5   8   5.62297
#
# LOCAL POTENTIAL
# lloc, lpopt,  rc(5),   dvloc0
    4   5   2.89331      0.50000
#
# VANDERBILT-KLEINMAN-BYLANDER PROJECTORs
# l, nproj, debl
    0   2   1.14841
    1   2   1.10423
    2   2   1.17152
    3   2   1.22641
```

```
#
# MODEL CORE CHARGE
# icmod, fcfact, rcfact
    0   0.00000   0.00000
#
# LOG DERIVATIVE ANALYSIS
# epsh1, epsh2, depsh
   -5.00    7.00    0.02
#
# OUTPUT GRID
# rlmax, drl
    6.00    0.01
#


# ATOM AND REFERENCE CONFIGURATION
# atsym  z   nc   nv     iexc    psfile
  Bi 83.00   12    3       4      upf
#
#   n    l    f        energy (Ha)
    1    0    2.00
    2    0    2.00
    2    1    6.00
    3    0    2.00
    3    1    6.00
    3    2   10.00
    4    0    2.00
    4    1    6.00
    4    2   10.00
    4    3   14.00
    5    0    2.00
    5    1    6.00
    5    2   10.00
    6    0    2.00
    6    1    3.00
#
# PSEUDOPOTENTIAL AND OPTIMIZATION
# lmax
    3
#
#   l,   rc,     ep,   ncon, nbas, qcut
    0   3.00000  -0.52904    4    7   4.00000
    1   3.00000  -0.14947    4    7   4.00000
    2   2.50000  -0.94601    4    8   6.00000
    3   3.00000   0.25000    4    8   5.00000
#
# LOCAL POTENTIAL
# lloc, lpopt,  rc(5),   dvloc0
    4    3   2.50000      0.00000
#
# VANDERBILT-KLEINMAN-BYLANDER PROJECTORs
# l, nproj, debl
    0    2   1.00000
    1    2   0.97647
    2    2   1.15596
    3    2   1.00000
```

```
#
# MODEL CORE CHARGE
# icmod, fcfact, rcfact
   1   0.25000   0.00000
#
# LOG DERIVATIVE ANALYSIS
# epsh1, epsh2, depsh
  -2.00    3.00    0.02
#
# OUTPUT GRID
# rlmax, drl
   7.00    0.01
#


# ATOM AND REFERENCE CONFIGURATION
# atsym  z   nc   nv     iexc    psfile
  Sn 50.00    8    3       4      upf
#
#   n    l    f       energy (Ha)
    1    0    2.00
    2    0    2.00
    2    1    6.00
    3    0    2.00
    3    1    6.00
    3    2   10.00
    4    0    2.00
    4    1    6.00
    4    2   10.00
    5    0    2.00
    5    1    2.00
#
# PSEUDOPOTENTIAL AND OPTIMIZATION
# lmax
    2
#
#   l,   rc,     ep,   ncon, nbas, qcut
    0   2.78311   0.00000    5    8   2.52914
    1   2.90187   0.00000    5    8   4.90513
    2   3.33533   0.00000    5    8   6.53914
#
# LOCAL POTENTIAL
# lloc, lpopt,  rc(5),   dvloc0
    4    2   1.91321      2.00000
#
# VANDERBILT-KLEINMAN-BYLANDER PROJECTORs
# l, nproj, debl
    0    2   0.99967
    1    2   0.85384
    2    2   1.34528
#
# MODEL CORE CHARGE
# icmod, fcfact, rcfact
    0   0.00000   0.00000
#
# LOG DERIVATIVE ANALYSIS
```

```
# epsh1, epsh2, depsh
 -12.00   12.00    0.02
#
# OUTPUT GRID
# rlmax, drl
   6.00    0.01
#


# ATOM AND REFERENCE CONFIGURATION
# atsym  z   nc   nv     iexc    psfile
 I 53.00    8    3       4      upf
#
#   n    l    f        energy (Ha)
   1    0    2.00
   2    0    2.00
   2    1    6.00
   3    0    2.00
   3    1    6.00
   3    2   10.00
   4    0    2.00
   4    1    6.00
   4    2   10.00
   5    0    2.00
   5    1    5.00
#
# PSEUDOPOTENTIAL AND OPTIMIZATION
# lmax
   2
#
#   l,   rc,     ep,   ncon, nbas, qcut
   0   2.37802   0.00000    5    8   3.07072
   1   3.31509   0.00000    5    8   3.93841
   2   3.15687   0.00000    5    8   8.33670
#
# LOCAL POTENTIAL
# lloc, lpopt,  rc(5),   dvloc0
   4    3   1.66551      3.70000
#
# VANDERBILT-KLEINMAN-BYLANDER PROJECTORs
# l, nproj, debl
   0    2   1.60066
   1    2   1.13374
   2    2   1.87444
#
# MODEL CORE CHARGE
# icmod, fcfact, rcfact
   0   0.00000   0.00000
#
# LOG DERIVATIVE ANALYSIS
# epsh1, epsh2, depsh
  -5.00    3.00    0.02
#
# OUTPUT GRID
# rlmax, drl
   6.00    0.01
```

```
#

# ATOM AND REFERENCE CONFIGURATION
# atsym  z   nc   nv     iexc    psfile
  Br 35.00    6    2       4      upf
#
#   n    l    f        energy (Ha)
    1    0    2.00
    2    0    2.00
    2    1    6.00
    3    0    2.00
    3    1    6.00
    3    2   10.00
    4    0    2.00
    4    1    5.00
#
# PSEUDOPOTENTIAL AND OPTIMIZATION
# lmax
    2
#
#   l,   rc,     ep,   ncon, nbas, qcut
    0   2.48883   0.00000    5    8   5.10687
    1   2.48044   0.00000    5    8   4.46675
    2   2.47352   0.09432    5    8   4.91674
#
# LOCAL POTENTIAL
# lloc, lpopt,  rc(5),   dvloc0
    4    2   2.24325      0.00000
#
# VANDERBILT-KLEINMAN-BYLANDER PROJECTORs
# l, nproj, debl
    0    2   1.26029
    1    2   1.41324
    2    2   1.05278
#
# MODEL CORE CHARGE
# icmod, fcfact, rcfact
    0   0.00000   0.00000
#
# LOG DERIVATIVE ANALYSIS
# epsh1, epsh2, depsh
  -15.00   15.00    0.02
#
# OUTPUT GRID
# rlmax, drl
    6.00    0.01
#


# ATOM AND REFERENCE CONFIGURATION
# atsym  z   nc   nv     iexc    psfile
  Cl 17.00    3    2       4      upf
#
#   n    l    f        energy (Ha)
    1    0    2.00
    2    0    2.00
```

```
   2    1    6.00
   3    0    2.00
   3    1    5.00
#
# PSEUDOPOTENTIAL AND OPTIMIZATION
# lmax
   1
#
#   l,   rc,      ep,   ncon, nbas, qcut
   0   3.19316   0.00000    5    8   6.06131
   1   1.60026   0.00000    5    8   6.97943
#
# LOCAL POTENTIAL
# lloc, lpopt,  rc(5),   dvloc0
   4    3   0.79857      0.00000
#
# VANDERBILT-KLEINMAN-BYLANDER PROJECTORs
# l, nproj, debl
   0    2   0.35558
   1    2   3.72254
#
# MODEL CORE CHARGE
# icmod, fcfact, rcfact
   0   0.00000   0.00000
#
# LOG DERIVATIVE ANALYSIS
# epsh1, epsh2, depsh
  -5.00    3.00    0.02
#
# OUTPUT GRID
# rlmax, drl
   6.00    0.01
#


# ATOM AND REFERENCE CONFIGURATION
# atsym  z   nc   nv     iexc    psfile
  Cs 55.00    9    3       4      upf
#
#   n    l    f        energy (Ha)
   1    0    2.00
   2    0    2.00
   2    1    6.00
   3    0    2.00
   3    1    6.00
   3    2   10.00
   4    0    2.00
   4    1    6.00
   4    2   10.00
   5    0    2.00
   5    1    6.00
   6    0    1.00
#
# PSEUDOPOTENTIAL AND OPTIMIZATION
# lmax
   2
```

```
#
#   l,   rc,     ep,   ncon, nbas, qcut
    0   2.55092   0.00000    5    8   4.59617
    1   2.28842   0.00000    5    8   6.06010
    2   2.35811   0.04706    5    8   4.28019
#
# LOCAL POTENTIAL
# lloc, lpopt,  rc(5),   dvloc0
    4    2   1.77341      1.00000
#
# VANDERBILT-KLEINMAN-BYLANDER PROJECTORs
# l, nproj, debl
    0    2   0.00000
    1    2   1.86520
    2    2   1.81189
#
# MODEL CORE CHARGE
# icmod, fcfact, rcfact
    0   0.00000   0.00000
#
# LOG DERIVATIVE ANALYSIS
# epsh1, epsh2, depsh
  -12.00   12.00    0.02
#
# OUTPUT GRID
# rlmax, drl
    6.00    0.01
#


# ATOM AND REFERENCE CONFIGURATION
# atsym  z   nc   nv     iexc    psfile
  Ag 47.00    6    4       4      upf
#
#   n    l    f        energy (Ha)
    1    0    2.00
    2    0    2.00
    2    1    6.00
    3    0    2.00
    3    1    6.00
    3    2   10.00
    4    0    2.00
    4    1    6.00
    5    0    2.00
    4    2    9.00
#
# PSEUDOPOTENTIAL AND OPTIMIZATION
# lmax
    2
#
#   l,   rc,     ep,   ncon, nbas, qcut
    0   2.63210  -3.64322    5    8   5.98964
    1   2.54829  -2.23885    5    8   6.43182
    2   2.45255  -0.38487    5    8   7.30643
#
# LOCAL POTENTIAL
```

```
# lloc, lpopt,  rc(5),   dvloc0
    4    5   1.52429      0.00000
#
# VANDERBILT-KLEINMAN-BYLANDER PROJECTORs
# l, nproj, debl
    0    2   3.43918
    1    2   2.19551
    2    2   1.48664
#
# MODEL CORE CHARGE
# icmod, fcfact, rcfact
    0   0.00000   0.00000
#
# LOG DERIVATIVE ANALYSIS
# epsh1, epsh2, depsh
   -5.00    3.00    0.02
#
# OUTPUT GRID
# rlmax, drl
    6.00    0.01
#
```
